# Supplementary material for: FedDr+: Stabilizing Dot-regression with Global Feature Distillation for Federated Learning
Source: arXiv:2406.02355 source file (2024-06-04)
Supplement: Supplementary file 1 [file analysis.tex]

\clearpage
\section{Additional Experiments}
\label{app:add_exp}
\subsection{Weight Norm Does Not Matter on FedFN}
We investigate the impact of increased data heterogeneity on weight norm disparity in the case of FedFN. Focusing on the $s$=2 setting, representing the most heterogeneous scenario, as shown in Figure~\ref{appfig:weight_norm_bias_fn}, we explore the evolution of weight norms between global and local models. During early training stages, a noticeable weight norm bias emerges within local models, favoring seen (ID) classes over unseen (OOD) classes. However, this bias progressively diminishes as the learning rate decreases, eventually aligning local models with the weight norm mean of the global model.

Additionally, we analyze variations in weight norm means between local models on the ID classes and the global model on the total classes under varying data heterogeneity. Specifically, we consider $s \in \{2, 5, 10\}$ and IID (Exactly class-balanced data distribution across clients) on the CIFAR-10 dataset. As illustrated in Figure~\ref{appfig:weight_norm_disparity_fn}, during initial training phases, the norm disparity between the global model and local models increases with data heterogeneity (i.e., IID $\rightarrow$ $s$=10 $\rightarrow$ $s$=5 $\rightarrow$ $s$=2). However, this disparity gradually diminishes across all settings as the learning rate decreases.

\newpage
\subsection{Additional GFL Results}

In the main paragraph of Section~\ref{sec:exp}, we report results exclusively in a balanced environment, specifically in the sharding setting. Table~\ref{tab:gfl_acc_all} presents results encompassing an unbalanced environment, specifically in the LDA setting. The reported outcomes stem from implementations with a consistent and identical seed, deviating from the context of the paragraph. In contrast to the main paragraph, we observe that in the MobileNet on CIFAR-100 environment with the $s=10$ setting, all baseline algorithms exhibit notably lower performance for the seed used in Table~\ref{tab:gfl_acc_all}. However, when applying the BABU or FN module, the performance difference is less pronounced, showing a more stable outcome than the main paragraph. Furthermore, consistently across all settings, applying the FN module to the baseline consistently demonstrates superior performance.

\begin{table}[h!]
    \centering
    \vspace{-0.15 in}
    \caption{FL Accuracy Comparison for Baseline, +BABU, and +FN.}
    \small
    \resizebox{1.0\textwidth}{!}{
    \begin{tabular}{cc|cccc|cccc|ccc|cccc}
      \toprule 
      \multirow{2.5}{*}{Algorithm} & \multirow{2.5}{*}{Module} & \multicolumn{8}{c|}{VGG11 on CIFAR-10} & \multicolumn{7}{c}{MobileNet on CIFAR-100} \\ \cmidrule{3-17}
      & & $s$=2 & $s$=3 & $s$=5 & $s$=10 & $\alpha$=0.1 & $\alpha$=0.3 & $\alpha$=0.5 & $\alpha$=1.0 & $s$=10 & $s$=50 & $s$=100 & $\alpha$=0.1 & $\alpha$=0.3 & $\alpha$=0.5 & $\alpha$=1.0 \\ \midrule
      & Baseline  & 73.83 & 78.99 & 81.40 & 82.79 & 73.16 & 80.77 & 81.63 & 82.45 & 26.64 & 40.18 & 41.50 & 42.66 & 42.68 & 43.82 & 41.57  \\ 
      FedAVG  & + BABU & 74.31 & 78.88 & 81.17 & 82.37  & 72.42 & 80.59 & 80.94 & 82.93 &  43.96 & 39.94 & 40.37 & 42.99 & 39.61 & 39.53 & 39.58  \\ 
      & \textbf{+ FN} & \textbf{77.23} & \textbf{81.46} & \textbf{82.80} & \textbf{84.16}  & \textbf{75.58} & \textbf{81.85} & \textbf{83.06} & \textbf{83.65} & \textbf{45.16} & \textbf{48.83} & \textbf{49.54} & \textbf{47.87} & \textbf{47.66} & \textbf{47.86} & \textbf{47.80}  \\  \midrule
      
      & Baseline & 77.07 & (\textit{Failed}) & \textbf{84.50} & 85.28 & (\textit{Failed}) & 83.24 & 83.54 & 85.21 & 34.64 & 42.56 & 43.67 & \textbf{45.18} & 45.62 & 44.42 & 43.16  \\
      Scaffold & + BABU & 76.89 & 82.24 & 84.26 & 85.02 & (\textit{Failed}) & 82.95 & 84.12 & 85.06 & 46.80 & 42.73 & 44.50 & 43.28 & 43.76 & 44.37 & 44.20 \\ 
       & \textbf{+ FN} & \textbf{79.05} & \textbf{82.83} & \textbf{84.80} & \textbf{85.83} & \textbf{74.53} & \textbf{83.65} & \textbf{84.79} & \textbf{85.42} & \textbf{50.17} & \textbf{48.74} & \textbf{51.04} & 45.10 & \textbf{49.71} & \textbf{50.42} & \textbf{52.13}  \\  \midrule

      % & Baseline & 71.87 & 77.14 & 79.27 & 81.81 & 70.85 & 79.12 & 80.28 & 82.17 & 25.14 & 40.53 & 42.87 & 40.59 & 42.59 & 43.61 & 43.15 \\
      % FedNTD & + BABU & 72.43 & 78.41 & 79.82 & 81.07 & 72.65 & 79.67 & 80.68 & 81.88 & 39.26 & 39.59 & 40.04 & 43.15 & 40.65 & 39.83 & 40.21 \\ 
      %  & \textbf{+ FN} & 68.07 & 75.02 & 77.34 & 81.18 & 64.69 & 76.79 & 79.30 & 80.77 & 38.97 & 47.36 & 49.69 & 45.54 & 47.48 & 48.29 & 48.40   \\  \midrule
       
      & Baseline & 73.92 & 78.86 & 81.47 & 82.61 & 73.39 & 80.94 & 81.16 & 82.64 & 26.57 & 39.93 & 42.11 & 42.71 & 42.77 & 44.54 & 41.55 \\
      FedEXP & +BABU & 74.48 & 78.91 & 81.16 & 82.17 & 71.61 & 80.50 & 81.24 & 82.72 & 45.44 & 41.49 & 40.24 & 42.73 & 40.09 & 39.54 & 40.66  \\ 
      & \textbf{+ FN} & \textbf{77.17} & \textbf{80.92} & \textbf{82.79} & \textbf{83.57} & \textbf{75.03} & \textbf{82.29} & \textbf{83.12} & \textbf{83.36} & \textbf{45.37} & \textbf{48.45} & \textbf{49.80} & \textbf{47.73} & \textbf{47.16} & \textbf{48.32} & \textbf{48.01} \\  \bottomrule 
    \end{tabular}
    }
    \label{tab:gfl_acc_all}
\end{table}
% \newpage
\subsection{Personalized Federated Learning (PFL) Results}\label{subsec:pfl_result}

We present FedFN-FT, a fine-tuned algorithm for PFL, inspired by prior work~\cite{oh2021fedbabu, dong2022spherefed}, utilizing local data. We compare FedFN-FT with existing PFL methods, including simple local models, 1-step approaches like FedPer~\cite{arivazhagan2019federated}, Per-FedAVG~\cite{fallah2020personalized}, and FedRep~\cite{collins2021exploiting}, as well as 2-step methods such as FedAVG-FT, FedBABU-FT~\cite{oh2021fedbabu}, SphereFed-FT (CE, MSE)\cite{dong2022spherefed}. Table~\ref{apptab:pfl_acc} provides detailed personalized accuracy results. The entries form of X±Y represents the mean and standard deviation of personalized accuracies across all clients for PFL algorithms. Entries without standard deviation indicate performance on $D_{test}$, derived from the global model after the initial step of 2-step methods.

Regarding the SphereFed, it constructs each element of the logit vector based on the cosine similarity between feature vectors and classifiers. Similar to FedFN, SphereFed necessitates rescaling the learning rate for classifier weights, leading to the need for separate learning rate tuning. To address this requirement,  we conduct an extensive grid search to determine the appropriate initial learning rate, denoted as $\eta$. Further details about the grid search are provided in Section~\ref{app:grid search}. 

For SphereFed (CE), SphereFed (MSE), and FedFN, we initialize the learning rates with $\eta$ values of 0.3, 4.5, and 0.5, respectively. The 2-step fine-tuning methods undergo a total of 5 local epochs, during which the learning rate was carried out through grid search within the range of $\{\eta, 0.1\times\eta, 0.01\times\eta\}$. The comprehensive results of the grid search for SphereFed and FN, including learning rate adjustments, are confirmed to be available in Appendix~\ref{app:finetuneing_lr_search}. Table~\ref{apptab:pfl_acc} documents the resulting tunned learning rates. In summary, 2-step methods consistently outperform 1-step methods regarding PFL performance. Among the 2-step methods, FedFN-FT consistently exhibits superior performance.

\begin{table}[htp]
    \centering
    \caption{PFL Accuracy Comparison for MobileNet on CIFAR-100.}
    \small
    \begin{tabular}{l|ccc}
    \toprule
    Algorithm & $s$=10 & $s$=50 & $s$=100 \\ \midrule
    Local only                              & 58.64{\tiny $\pm$7.21}  & 25.38{\tiny $\pm$4.12} & 18.52{\tiny $\pm$3.15} \\ \midrule
    FedPer (2019)                           & 70.92{\tiny $\pm$6.93}  & 33.73{\tiny $\pm$4.68} & 22.77{\tiny $\pm$4.30} \\
    Per-FedAVG (2020)                       & 32.57{\tiny $\pm$11.02} & 43.09{\tiny $\pm$7.36} & 45.00{\tiny $\pm$7.05} \\
    FedRep (2021)                           & 62.69{\tiny $\pm$7.26}  & 34.66{\tiny $\pm$5.34} & 26.53{\tiny $\pm$4.52} \\ \midrule
    FedAVG (2017)                           & 36.30 & 41.97   & 42.51 \\ 
    FedAVG-FT (0.1$\times\eta$)             & 77.39{\tiny $\pm$6.40}  & 50.57{\tiny $\pm$5.31} & 46.95{\tiny $\pm$4.90} \\
    FedBABU (2022)                          & 45.73 & 39.57   & 40.70  \\
    FedBABU-FT (0.01$\times\eta$)           & 79.76{\tiny $\pm$6.05}  & 50.93{\tiny $\pm$4.69} & 46.63{\tiny $\pm$5.25} \\
    SphereFed (CE) (2022)                   & 40.39 & 43.68   & 44.96 \\ 
    SphereFed-FT (CE) (0.1$\times\eta$)     & 77.24{\tiny $\pm$6.38}  & 55.08{\tiny $\pm$5.33} & 50.17{\tiny $\pm$5.04} \\ 
    SphereFed (MSE) (2022)                  & 43.42 & 48.05   & 49.51 \\ 
    SphereFed-FT (MSE) (0.01$\times\eta$)   & \textbf{82.50}{\tiny $\pm$6.04} & 56.45{\tiny $\pm$5.56} & 53.10{\tiny $\pm$4.90}   \\ \midrule
    FedFN                                   & 46.98 & 49.47   & 50.92 \\
    \textbf{FedFN-FT} (0.1$\times\eta$)     & \textbf{82.85}{\tiny $\pm$5.83} & \textbf{60.78}{\tiny $\pm$4.99} & \textbf{55.43}{\tiny $\pm$5.24} \\
    \bottomrule
    \end{tabular}
    \label{apptab:pfl_acc}
\end{table}
\newpage

\subsubsection{Fine Tuning Learning Rate Search}\label{app:finetuneing_lr_search}
\begin{table*}[h!]
  \centering  
  \caption{Search for Finetuning Learning Rates in Two-Step Methods.}
\resizebox{0.8\textwidth}{!}{%
\begin{tabular}{c|ccc}
\toprule
Algorithm &  $s$=10 & $s$=50 & $s$=100  \\ \midrule

FedAVG (2017) & 36.30    & 41.97    & 42.51        \\ 

FedAVG-FT ($\eta$) & 67.23 $\pm$ 6.32 & 35.98 $\pm$ 5.56 & 38.25 $\pm$ 5.29    \\ 

\textbf{FedAVG-FT} (0.1$\times\eta$) & \textbf{77.39 $\pm$ 6.40} & \textbf{50.57 $\pm$ 5.31} & \textbf{46.95 $\pm$ 4.90} \\

FedAVG-FT (0.01$\times\eta$) & 70.96 $\pm$ 6.81   & 44.78 $\pm$ 4.88   & 44.00 $\pm$ 4.93       \\ 
\midrule

FedBABU (2022) & 45.73 & 39.57  & 40.7  \\ 

FedBABU-FT ($\eta$) & 13.32 $\pm$ 4.51   & 4.72 $\pm$ 1.85   & 2.85 $\pm$ 1.27       \\ 

FedBABU-FT (0.1$\times\eta$) & 77.88 $\pm$ 6.59 & 51.75 $\pm$ 4.84 & 46.02 $\pm$ 5.24 \\ 

\textbf{FedBABU-FT} (0.01$\times\eta$) & \textbf{79.76 $\pm$ 6.05} & \textbf{50.93 $\pm$ 4.69} & \textbf{46.63 $\pm$ 5.25} \\ \midrule

SphereFed (CE) (2022) & 40.39  & 43.68  & 44.96  \\ 

SphereFed-FT (CE) ($\eta$) & 53.79 $\pm$ 9.47 & 32.11 $\pm$ 6.89 & 27.81 $\pm$ 4.98 \\ 

\textbf{SphereFed-FT (CE)} (0.1$\times\eta$) & \textbf{77.24 $\pm$ 6.38}   & \textbf{55.08 $\pm$ 5.33} & \textbf{50.17 $\pm$ 5.04} \\ 

SphereFed-FT (CE) (0.01$\times\eta$) & 77.18 $\pm$ 6.17 & 49.99 $\pm$ 4.79   & 47.45 $\pm$ 4.70       \\

\midrule

SphereFed (MSE) (2022) & 43.42  & 48.05  & 49.51  \\ 

SphereFed-FT (MSE) ($\eta$) & 57.34 $\pm$ 7.53 & 35.43 $\pm$ 5.32 & 27.95 $\pm$ 5.03 \\ 

SphereFed-FT (MSE) (0.1$\times\eta$) & 79.73 $\pm$ 6.63 & 56.80 $\pm$ 5.29 & 51.06 $\pm$ 5.59 \\ 

\textbf{SphereFed-FT (MSE)} (0.01$\times\eta$) & \textbf{82.50 $\pm$ 6.04} & \textbf{56.45 $\pm$ 5.56} & \textbf{53.10 $\pm$ 4.90} \\ 
\midrule
FedFN  & 46.98 & 49.47 & 50.92  \\

FedFN-FT ($\eta$) & 71.88 $\pm$ 6.73 & 43.80 $\pm$ 4.54 & 41.23 $\pm$ 5.46       \\ 

\textbf{FedFN-FT} (0.1$\times\eta$) & \textbf{82.85 $\pm$ 5.83}   & \textbf{60.78 $\pm$ 4.99} & \textbf{55.43 $\pm$ 5.24}    \\

FedFN-FT (0.01$\times\eta$) & 82.15 $\pm$ 5.74 & 54.24 $\pm$ 5.06 & 51.92 $\pm$ 5.06    \\ 
\bottomrule
   
        \end{tabular}%
    }
\label{tab:2_step_fine_tune_lr_search}
\end{table*}

\newpage
\subsection{Logit Should Be Non-Restricted}
SphereFed~\cite{dong2022spherefed} modifies i-th index of the logit vector of an input $x$, represented as $\tilde{z}_{i}(x;\theta)=\tilde{\theta}_{cls, i}\frac{f(x;\theta_{ext})}{||f(x;\theta_{ext})||_{2}}$. It maintains the classifier $\Tilde{\theta}_{cls}$ in a frozen state, ensuring that the norms of $\Tilde{\theta}_{cls, i}$ are orthonormal to each other. As a result, $\tilde{z}_{i}(x;\theta)$ becomes the cosine similarity between $f(x;\theta_{ext})$ and $\tilde{\theta}_{cls, i}$, yielding values restricted to the range [-1,1]. Following this modification, the logit margin is constrained to a maximum value of 2.

As seen in Table~\ref{apptab:pfl_acc}, SphereFed (CE) performs inferior to even FedBABU despite utilizing feature normalization. We propose modifying the SphereFed (CE) logit vector to address this limitation. We transform it to $\tilde{z}^{\tau}_{i}(x;\theta)=\tau\,\tilde{\theta}_{cls, i}\frac{f(x;\theta_{ext})}{||f(x;\theta_{ext})||_{2}}$, which yields values in the range of [-$\tau$, $\tau$], providing less constrained outputs. We apply this approach with different values of $\tau$, specifically $\{10, 15, 20, 25, 30\}$, in the $s$=10 setting. We compared the results of this modified SphereFed (CE) with those of SphereFed (MSE), FedBABU, and FedFN, and the outcomes are presented in Table~\ref{apptab:modified_spherefed}.
Increasing $\tau$ up to 15 results in improvements in SphereFed(CE), although not as significant as FedFN. However, it shows enhancements over FedBABU and SphereFed(MSE) at 15. Consequently, this indicates that creating the logit vector through feature normalization with relaxed constraints on the elements of the logit is recommended.
 
\begin{table}[h!]
\centering
\caption{Comparison of Modified SphereFed (CE) with SphereFed (MSE), FedBABU, and FedFN on $s$=10 Setting of CIFAR-100.}
\resizebox{0.4\textwidth}{!}{
\begin{tabular}{c|c}
\toprule
Algorithm & Accuracy \\ \midrule
SphereFed (CE), $\tau$=1 & 40.39 \\   
SphereFed (CE), $\tau$=10  & 42.84 \\ 
SphereFed (CE), $\tau$=15  & \textbf{45.78} \\ 
SphereFed (CE), $\tau$=20  & 44.95 \\ 
SphereFed (CE), $\tau$=25  & 44.46 \\ 
SphereFed (CE), $\tau$=30  & 39.62 \\  \midrule
SphereFed (MSE)  & 43.42 \\\midrule
FedBABU  & 45.73 \\ \midrule
FedFN  & \textbf{46.98} \\
\bottomrule
\end{tabular}
}
\label{apptab:modified_spherefed}
\end{table}

\newpage
\subsection{Reproduced Result from SphereFed}

We present the experimental results for SphereFed~\cite{dong2022spherefed} trained with LDA settings ($\alpha\in\{0.1, 0.5\}$) on CIFAR-100. To reproduce the experiments presented in the original paper, we deviated from our previous experimental settings. Specifically, for the MobileNetV2 model architecture, we constructed the layers exactly as described in Table 7 of \citep{dong2022spherefed}. Regarding the training setup, each case is trained for 500 rounds using cosine annealing, following the guidelines of the original paper. We also follow the original paper's instructions for all other hyperparameters. It should be noted that we did not employ the FFC algorithm in any of the experiments, including those using FedAVG and FedFN.

Table~\ref{apptab:spherefed_reproduce} presents the new results we obtain and compares them with the original outcomes of SphereFed, encompassing FedAVG, FedFN, and centralized learning. If certain algorithms are not indicated in the original results, we represent them with a dash (``-"). For the algorithms implemented as described in the original paper, we provide specific details like the actual learning rate $\eta$. Furthermore, for each FL algorithm, we present reproduced results across a specified range of initial learning rates $\eta\in\{0.1, 0.3, 0.5, 1.0, 1.5, 3.0, 4.5, 5.0\}$. In the case of centralized learning, results are provided explicitly for $\eta=0.1$.

Following this, we conclude that the original paper's results could not be reproduced. The reported performance of FL algorithms in the actual original paper (71.85, 68.78) appears surprisingly higher than the reproduced results in centralized learning (68.27). Moreover, implementing the algorithms with the exact settings reported in the original results consistently leads to lower performance (71.85 vs 18.01, 68.78 vs 37.76). Even when implemented following the specifications of the original paper ($\eta$=0.5), SphereFed (MSE) demonstrated significantly poor performance at 18.01. Subsequently, despite a thorough investigation through grid search, the best-performing configuration obtained is 52.69, still falling below the reported performance. Furthermore, when comparing the performance at the optimal learning rate for each FL algorithm, we consistently observe that FedFN outperforms the baselines.

\begin{table}[h!]
    \centering
    \caption{Reproduced Results for SphereFed, FedAVG, and FedFN under the Same Settings, Utilizing MobileNet (as Described in \citep{dong2022spherefed}) on CIFAR-100.}

    \resizebox{\textwidth}{!}{
        \begin{tabular}{c|cccccccc|c}
        \toprule
        \emph{SphereFed (MSE)} & \emph{$\eta$=0.1} & \emph{$\eta$=0.3} & \emph{$\eta$=0.5} & \emph{$\eta$=1.0} & \emph{$\eta$=1.5} & \emph{$\eta$=3.0} & \emph{$\eta$=4.5} & \emph{$\eta$=5.0} & Original Result (\emph{$\eta$=0.5})   \\ \cmidrule{1-10}         
        $\alpha$=0.5 & 2.77 & 9.73 & 18.01 & 43.26 & 52.19 & \textbf{52.69} & 48.20 & 40.87 & 71.85 \\
        $\alpha$=0.1 & 2.88 & 9.65 & 20.19 & 41.48 & 45.41 & \textbf{46.34} & 43.62 & 40.56 & - \\ \midrule
        \emph{SphereFed (CE)} & \emph{$\eta$=0.1} & \emph{$\eta$=0.3} & \emph{$\eta$=0.5} & \emph{$\eta$=1.0} & \emph{$\eta$=1.5} & \emph{$\eta$=3.0} & \emph{$\eta$=4.5} & \emph{$\eta$=5.0} & Original Result   \\ \cmidrule{1-10}         
        $\alpha$=0.5 & 37.57 & 49.39 & 48.18 & 52.51 & \textbf{52.99} & 51.09 & 44.87 & 44.23 & - \\
        $\alpha$=0.1 & 22.37 & 40.58 & 42.85 & 40.92 & \textbf{47.72} & 42.11 & 35.30 & 33.83 & - \\ \midrule
        \emph{FedAVG} & \emph{$\eta$=0.1} & \emph{$\eta$=0.3} & \emph{$\eta$=0.5} & \emph{$\eta$=1.0} & \emph{$\eta$=1.5} & \emph{$\eta$=3.0} & \emph{$\eta$=4.5} & \emph{$\eta$=5.0} & Original Result (\emph{$\eta$=0.1})   \\ \cmidrule{1-10}         
        $\alpha$=0.5 & 37.76 & \textbf{38.82} & 23.76 & 1.04 & 1.02 & 1.03 & 1.25 & 1.01 & 68.78 \\
        $\alpha$=0.1 & 38.58 & \textbf{40.47} & 27.35 & 1.22 & 1.04 & 1.02 & 1.09 & 1.17 & - \\ \midrule
        \emph{FedFN} & \emph{$\eta$=0.1} & \emph{$\eta$=0.3} & \emph{$\eta$=0.5} & \emph{$\eta$=1.0} & \emph{$\eta$=1.5} & \emph{$\eta$=3.0} & \emph{$\eta$=4.5} & \emph{$\eta$=5.0} & Original Result   \\ \cmidrule{1-10}         
        $\alpha$=0.5 & 55.00 & \textbf{53.38} & 48.55 & 49.89 & 45.79 & 42.45 & 35.43 & 34.82 & - \\
        $\alpha$=0.1 & 46.38 & \textbf{49.16} & 46.61 & 41.69 & 42.03 & 38.80 & 30.92 & 2.89 & - \\ \midrule
        \emph{Centralized Learning} &   \multicolumn{8}{c|}{\textbf{68.27} (\emph{$\eta$=0.1})} & - \\ \bottomrule

        \end{tabular}
        }
        \label{apptab:spherefed_reproduce}
\end{table}

\newpage
\subsection{FedFN vs FedFR}

We compare the performance of FedFN with Federated Averaging with Feature Norm Regularization (FedFR) introduced in Eq.~\eqref{eqn:fedfr} in the main paragraph. Table~\ref{apptab:cifar10_fedfr} and Table~\ref{apptab:cifar100_fedfr} present the performance on CIFAR-10 and CIFAR-100 with $s=10$ setting, respectively.

Table~\ref{apptab:cifar10_fedfr} reports results of FedFR on CIFAR-10, referring to the optimal hyperparameter $\mu=0.005$ from Figure~\ref{fig:fedfr-result} in the main paragraph. FedFR exhibits slightly lower performance compared to FedFN but demonstrates superiority over FedAVG and FedBABU. In the $s=10$ setting of CIFAR-100, FedFR shows comparable or superior performance to FedAVG. However, FedFR performs worse than both FedBABU and FedFN across all hyperparameter candidates. In contrast to FedFR, FedFN consistently demonstrates superior performance across all settings.

\begin{table}[htp]
    \centering
    \vspace{-0.15 in}
    \caption{Accuracy Comparison on CIFAR-10.}
    \small
    \begin{tabular}{c|cccc}
    \toprule
    \multirow{2.5}{*}{Algorithm} & \multicolumn{4}{c}{VGG11 on CIFAR-10}\\ \cmidrule{2-5} 
                                 & $s$=2 & $s$=3 & $s$=5 & $s$=10 \\ \midrule
    FedAVG   & 74.24 & 77.29 & 81.08 & 81.97  \\ 
    FedBABU   & 75.05 & 77.73 & 81.04 & 82.16  \\     
    FedFR  & 76.14 & 77.89 & 81.61 & 82.18 \\ 
    FedFN    & \textbf{77.77} & \textbf{78.93} & \textbf{82.43} & \textbf{83.80} \\ \bottomrule                            
    \end{tabular}    \label{apptab:cifar10_fedfr}
\end{table}

\begin{table}[h!]
    \centering
    \caption{Accuracy Comparison on the $s=10$ Setting of MobileNet on CIFAR-100.}
    \resizebox{\textwidth}{!}{
        \begin{tabular}{c|cccccccc}
        \toprule
        \multirow{2.5}{*}{FedFR} & \emph{$\mu$=0.5} & \emph{$\mu$=0.1} &\emph{$\mu$=0.05} & \emph{$\mu$=0.01} & \emph{$\mu$=0.005} & \emph{$\mu$=0.001} & \emph{$\mu$=0.0005} & \emph{$\mu$=0.0001}\\ \cmidrule{2-9}         
          & \emph{(Failed)} & 37.74 & \textbf{39.50} & 36.72 & 36.51 & 36.77 & 37.04 & 37.30\\ \midrule
        FedAVG &   \multicolumn{8}{c}{\textbf{36.30} (\emph{$\mu$=0.0})} \\ \midrule
        FedBABU &   \multicolumn{8}{c}{\textbf{45.73}} \\ \midrule
        FedFN &   \multicolumn{8}{c}{\textbf{46.98}} \\ \bottomrule
        
        \end{tabular}
        }
        \label{apptab:cifar100_fedfr}
\end{table}
\newpage
\subsection{FN in the Centralized Learning}
\begin{figure}[h!]
    \centering    
    \includegraphics[width=1.0\textwidth]{fig/cifar100_centralized_test_accuracy_plot.png}
    \caption{Module Comparison in Centralized Learning}
    \label{fig:centralized_acc_cifar100}
\end{figure}
In FedBABU~\cite{oh2021fedbabu}, the authors comprehensively evaluate the performance of the Full and Body modules in a centralized learning setup. Expanding upon their analysis, we incorporate the FN module to assess its performance compared to the Full and Body modules. We replicate the experimental settings outlined in \cite{oh2021fedbabu} to ensure fair comparisons. The experiments are carried out on the CIFAR-100 dataset, utilizing the MobileNet architecture. The results of the conducted experiments are depicted in Figure~\ref{fig:centralized_acc_cifar100}.

As expected, our evaluation reveals a slight decline in performance within the Body module compared to the Full module, aligning with the findings reported in \cite{oh2021fedbabu}. This performance difference can be attributed to the partial update constraint imposed on the model during the training of the Body module. In contrast, despite incorporating the constraint of feature normalization, the FN module exhibits significant improvements over the Full module. This enhancement is attributed to the capacity of the FN module to empower the model to acquire more effective and discriminative representations, thereby enhancing overall performance.
