# Supplementary material for: FedDr+: Stabilizing Dot-regression with Global Feature Distillation for Federated Learning
Source: arXiv:2406.02355 source file (2024-06-04)
Supplement: Supplementary file 2 [file grid_search.tex]

\iffalse
\subsection{FedBABU vs. FedAVG vs. FedETF}
We conduct grid searches for FedAVG~\cite{mcmahan2017communication}, FedBABU~\cite{oh2021fedbabu}, and FedETF. Table ~\ref{apptab:grid_mobile} to ~\ref{apptab:grid_vgg} present the grid search results for VGG on CIFAR-10, MobileNet on CIFAR-100, ResNet18 on CIFAR-10, and Pretrained ResNet18 on CIFAR-10, respectively. In these tables, we abbreviate FedAVG, FedBABU, and FedFN as AVG, BABU, and FN, respectively, and indicate cases where the final global model fails to converge during training with a ``-" in the respective table cells. The determined optimal hyperparameter $\eta$ values for FedFN are as follows: 0.03, 0.5, 0.1, and 0.1 for Table ~\ref{apptab:grid_mobile} to ~\ref{apptab:grid_vgg}, respectively.

\begin{table}[htp]
    \centering
    \caption{Grid Search Results for MobileNet on CIFAR-100.}
    \label{apptab:grid_mobile}
    \resizebox{0.8\textwidth}{!}{
        \begin{tabular}{c|ccc|ccc|ccc|ccc}
        \toprule
        \multirow{2.5}{*} {\emph{$\eta$=0.1}} & \multicolumn{3}{c|}{$E$=1} & \multicolumn{3}{c|}{$E$=3} & \multicolumn{3}{c|}{$E$=5} & \multicolumn{3}{c}{$E$=10} \\ \cmidrule{2-13}         
        & BABU & AVG & ETF  & BABU & AVG & ETF  & BABU & AVG & ETF  & BABU & AVG & ETF   \\ \midrule           
        $s$=100 & 41.32 & 41.57 & 40.25 & \textbf{46.34} & \textbf{46.29} & 46.86 & 40.49 & 43.19 & 40.17 & 37.03 & 38.13 & 36.68 \\ 
        
        $s$=50 & 40.86 & 38.35 & 36.36 & \textbf{44.40} & \textbf{45.32} & 44.16 & 40.76  &  40.63 & 40.93 & 36.79 & 37.77 & 35.94\\ 
        

        
        $s$=10 & 33.95 & 27.02 & 23.32 & \textbf{46.20} & \textbf{37.22} & 31.99 & 45.56 &  36.60 & 31.74 & 41.01 & 34.67 & 32.06 \\         
        % \midrule
        % \multirow{2}{*} {\emph{$\eta$=0.3}} & \multicolumn{3}{c|}{$E$=1} & \multicolumn{3}{c|}{$E$=3} & \multicolumn{3}{c|}{$E$=5} & \multicolumn{3}{c}{$E$=10} \\ \cmidrule{2-13}         
        % & BABU & AVG & ETF  & BABU & AVG & ETF  & BABU & AVG & ETF  & BABU & AVG & ETF   \\ \midrule    

        
        % $s$=100 & 46.65 & 41.76 & 42.59  & \textbf{45.88} & 50.59 & 47.61  & 40.57 & 46.67 & 42.89  & 37.79 & 41.28 & 36.46\\ 
        
        % $s$=50 & 44.03 & 37.83 & 40.13  & \textbf{45.57} & 48.79 & 47.04  & 40.02 & 45.28 & 42.14  & 37.28 & 42.65 & 37.07\\   

        
        % $s$=10 & 37.37 & 26.66 & 25.15  & \textbf{46.43} & 29.85 & 32.91   & 47.07 &  33.78 & 32.68  & 44.57 & 36.42 & 33.54  \\                  
        \midrule
        \multirow{2}{*} {\emph{$\eta$=0.5}} & \multicolumn{3}{c|}{$E$=1} & \multicolumn{3}{c|}{$E$=3} & \multicolumn{3}{c|}{$E$=5} & \multicolumn{3}{c}{$E$=10} \\ \cmidrule{2-13}         
        & BABU & AVG & ETF  & BABU & AVG & ETF  & BABU & AVG & ETF  & BABU & AVG & ETF   \\ \midrule  

        
        $s$=100 & 47.18 & 35.81 & 42.95 & 45.05 & - & \textbf{49.71} & 39.33 & - & 41.44 & 38.23 & - & 37.32  \\ 
        
        $s$=50 & 47.53 & 36.28 & 41.47  & 46.68 & 47.43 & \textbf{48.42}  & 40.42 & - & 43.38  & 37.71 & 44.76 & 38.96  \\   
        
        
        $s$=10 & 38.59 & 8.39 & 24.07 & 46.23 & 8.60 & \textbf{32.42} & 45.14 &  - & 32.57 & 44.03 & - & 34.29\\         
        
        \midrule
        
        \multirow{2}{*} {\emph{$\eta$=1.0}} & \multicolumn{3}{c|}{$E$=1} & \multicolumn{3}{c|}{$E$=3} & \multicolumn{3}{c|}{$E$=5} & \multicolumn{3}{c}{$E$=10} \\ \cmidrule{2-13}         
        & BABU & AVG & ETF  & BABU & AVG & ETF  & BABU & AVG & ETF  & BABU & AVG & ETF   \\ \midrule   

        
        $s$=100 & 46.92 & 31.15 & 43.12 & 45.28 & 23.84 & 49.72 & 39.61 & 34.66 & 43.65 & 37.12 & 42.06 & 38.57 \\ 
        
        $s$=50 & 45.24 & 26.64 & 38.96 & 47.99 & 14.79 & 49.25  & 40.11 & 28.02 & 44.02 & 38.76 & 39.47 & 39.67  \\    
        
        $s$=10 & 38.59 & 8.49 & 23.44 & 45.42 & 11.48 & 31.08  & 45.14 &  - & 32.13 & 44.03 & - & 34.23 \\         
        \bottomrule
    
    
        \end{tabular}
        }
\end{table}




\begin{table}[h!]
    \centering
    \caption{Grid Search Results for VGG11 on CIFAR-10.}
    \label{apptab:grid_vgg}
    \resizebox{0.9\textwidth}{!}{
        \begin{tabular}{c|ccc|ccc|ccc|ccc}
        \toprule
        \multirow{2.5}{*} {\emph{$\eta$=0.01}} & \multicolumn{3}{c|}{$E$=5} & \multicolumn{3}{c|}{$E$=10} & \multicolumn{3}{c|}{$E$=15} & \multicolumn{3}{c}{$E$=20}  \\ \cmidrule{2-13}         
        & BABU & AVG & ETF & BABU & AVG & ETF & BABU & AVG & ETF & BABU & AVG & ETF \\ \midrule  
        $s$=10 & 82.43 & 82.68 & 81.35 & \textbf{82.56} & \textbf{83.03} & 80.01 & 82.16 & 81.97 & 78.56 & 81.82 & 81.66 & 78.79 \\ 
        
        $s$=5 & 79.39 & 80.42 & 78.90  & \textbf{81.13} & \textbf{81.36} & 78.27 & 81.04 & 81.08 & 78.34 & 80.82 & 81.35 & 78.65 \\ 
        
        
        $s$=2 & 56.37 & 63.78 & 68.47 & \textbf{73.31} & \textbf{73.24} & 69.23 & 75.05 & 74.24 & 69.54 & 75.25 & 74.98 & 69.67 \\ \midrule
        
        % \multirow{2.5}{*} {\emph{$\eta$=0.03}} & \multicolumn{3}{c|}{$E$=5} & \multicolumn{3}{c|}{$E$=10} & \multicolumn{3}{c|}{$E$=15} & \multicolumn{3}{c}{$E$=20}  \\ \cmidrule{2-13}         
        % & BABU & AVG & ETF & BABU & AVG & ETF & BABU & AVG & ETF & BABU & AVG & ETF \\ \midrule     
        % $s$=10 & 84.23 & 84.32 & 82.65 & \textbf{84.10} & \textbf{84.13} & 82.17 & 83.61 & 84.38 & 82.34 & 83.82 & 83.42 & 81.34 \\ 
        
        % $s$=5 & 82.14 & 82.56 & 79.67 & \textbf{82.19} & \textbf{82.39} & 80.37 & 83.17 & 82.92 & 79.77 & 82.49 & 82.66 & 79.90 \\ 
        
        
        % $s$=2 & 50.80 & 62.80 & 67.11 & \textbf{74.27} & \textbf{75.08} & 67.18 & 74.57 & - & 68.43 & 77.36  & - & 69.94 \\ \midrule
        
        \multirow{2.5}{*} {\emph{$\eta$=0.05}} & \multicolumn{3}{c|}{$E$=5} & \multicolumn{3}{c|}{$E$=10} & \multicolumn{3}{c|}{$E$=15} & \multicolumn{3}{c}{$E$=20}  \\ \cmidrule{2-13}         
        & BABU & AVG & ETF & BABU & AVG & ETF & BABU & AVG & ETF & BABU & AVG & ETF \\ \midrule        
        $s$=10 & 84.49 & 84.51 & 82.62 & 84.22 & 84.30 & \textbf{82.75} & 84.19 & 84.18 & 82.45 & 83.94 & - & 81.83 \\ 
        
        $s$=5 & 81.74 & 81.62 & 80.04 & 82.77 & - & \textbf{80.11} & - & - & 80.06 & 82.90 & - & 80.30 \\ 
        
        
        $s$=2 & - & 61.66 & 66.89 & 71.52 & - & \textbf{67.51} & - & - & 68.52 & - & - & 68.58 \\ \midrule
        
        \multirow{2.5}{*} {\emph{$\eta$=0.1}} & \multicolumn{3}{c|}{$E$=5} & \multicolumn{3}{c|}{$E$=10} & \multicolumn{3}{c|}{$E$=15} & \multicolumn{3}{c}{$E$=20}  \\ \cmidrule{2-13}         
        & BABU & AVG & ETF & BABU & AVG & ETF & BABU & AVG & ETF & BABU & AVG & ETF \\ \midrule         

        $s$=10 & 83.90 & - & 82.64 & 84.05 & - & 82.36 & - & - & 81.56 & - & - & 81.52 \\ 
        
        $s$=5 & - & - & 79.16 & - & - & 80.03 & - & - & 79.29 & - & - & 79.07\\ 
        
        $s$=2 &  - & - & 60.85 & - & - & 56.43 & - & - & 63.66 & - & - & 57.97\\        
        
        
        \bottomrule
        
        \end{tabular}
        } 
\end{table}


\clearpage

\newpage
\subsection{Dot-Regression vs. Dot-Regression-FD}

\begin{table}[htp]
    \centering
    \caption{Grid Search Results for MobileNet on CIFAR-100.}
    \resizebox{0.6\textwidth}{!}{
        \begin{tabular}{c|cc|cc|cc|cc}
        \toprule
        \multirow{2.5}{*} {\emph{$\eta$=1.0}} & \multicolumn{2}{c|}{$E$=1} & \multicolumn{2}{c|}{$E$=3} & \multicolumn{2}{c|}{$E$=5} & \multicolumn{2}{c}{$E$=10} \\ \cmidrule{2-9}         
        & Dot & Dot-FD & Dot & Dot-FD & Dot & Dot-FD & Dot & Dot-FD \\ \midrule     

        
        $s$=100 & 0.00 & 0.00 & 49.51 & 40.74 & 0.00 & 0.00 & 0.00 & 0.00 \\ 
        
        $s$=50 & 0.00 & 0.00 & 45.70 & 46.89 & 0.00 & 0.00 & 0.00 & 0.00 \\ 
        

        
        $s$=10 & 0.00 & 0.00 & 40.74 & 42.15 & 0.00 & 0.00 & 0.00 & 0.00 \\ 
        \midrule
        
        \multirow{2.5}{*} {\emph{$\eta$=3.0}} & \multicolumn{2}{c|}{$E$=1} & \multicolumn{2}{c|}{$E$=3} & \multicolumn{2}{c|}{$E$=5} & \multicolumn{2}{c}{$E$=10} \\ \cmidrule{2-9}         
        & Dot & Dot-FD & Dot & Dot-FD & Dot & Dot-FD & Dot & Dot-FD \\ \midrule    

        
        $s$=100 & 0.00 & 0.00 & 48.66 & 51.74 & 0.00 & 0.00 & 0.00 & 0.00 \\ 
        
        $s$=50 & 0.00 & 0.00 & 49.74 & 50.38 & 0.00 & 0.00 & 0.00 & 0.00 \\ 
        

        
        $s$=10 & 0.00 & 0.00 & 42.86 & 49.05 & 0.00 & 0.00 & 0.00 & 0.00 \\ 
        \midrule

        \multirow{2.5}{*} {\emph{$\eta$=4.5}} & \multicolumn{2}{c|}{$E$=1} & \multicolumn{2}{c|}{$E$=3} & \multicolumn{2}{c|}{$E$=5} & \multicolumn{2}{c}{$E$=10} \\ \cmidrule{2-9}         
        & Dot & Dot-FD & Dot & Dot-FD & Dot & Dot-FD & Dot & Dot-FD \\ \midrule    

        
        $s$=100 & 0.00 & 0.00 & 51.72 & 50.55 & 0.00 & 0.00 & 0.00 & 0.00 \\ 
        
        $s$=50 & 0.00 & 0.00 & 51.00 & 51.26 & 0.00 & 0.00 & 0.00 & 0.00 \\ 
        

        
        $s$=10 & 0.00 & 0.00 & 41.27 & 48.14 & 0.00 & 0.00 & 0.00 & 0.00 \\ 
        \midrule
        

        
        \multirow{2.5}{*} {\emph{$\eta$=5.0}} & \multicolumn{2}{c|}{$E$=1} & \multicolumn{2}{c|}{$E$=3} & \multicolumn{2}{c|}{$E$=5} & \multicolumn{2}{c}{$E$=10} \\ \cmidrule{2-9}         
        & Dot & Dot-FD & Dot & Dot-FD & Dot & Dot-FD & Dot & Dot-FD \\ \midrule    

        
        $s$=100 & 0.00 & 0.00 & \textbf{52.86} & \textbf{53.23} & 0.00 & 0.00 & 0.00 & 0.00 \\ 
        
        $s$=50 & 0.00 & 0.00 & \textbf{53.57} & \textbf{51.49} & 0.00 & 0.00 & 0.00 & 0.00 \\ 
        

        
        $s$=10 & 0.00 & 0.00 & \textbf{42.52} & \textbf{48.69} & 0.00 & 0.00 & 0.00 & 0.00 \\ 
  
        \midrule

        \multirow{2.5}{*} {\emph{$\eta$=5.5}} & \multicolumn{2}{c|}{$E$=1} & \multicolumn{2}{c|}{$E$=3} & \multicolumn{2}{c|}{$E$=5} & \multicolumn{2}{c}{$E$=10} \\ \cmidrule{2-9}         
        & Dot & Dot-FD & Dot & Dot-FD & Dot & Dot-FD & Dot & Dot-FD \\ \midrule    

        
        $s$=100 & 0.00 & 0.00 & 51.87 & 53.43 & 0.00 & 0.00 & 0.00 & 0.00 \\ 
        
        $s$=50 & 0.00 & 0.00 & 51.00 & 51.83 & 0.00 & 0.00 & 0.00 & 0.00 \\ 
        

        
        $s$=10 & 0.00 & 0.00 & 43.65 & 47.04 & 0.00 & 0.00 & 0.00 & 0.00 \\ 
        \midrule

        \multirow{2.5}{*} {\emph{$\eta$=6.0}} & \multicolumn{2}{c|}{$E$=1} & \multicolumn{2}{c|}{$E$=3} & \multicolumn{2}{c|}{$E$=5} & \multicolumn{2}{c}{$E$=10} \\ \cmidrule{2-9}         
        & Dot & Dot-FD & Dot & Dot-FD & Dot & Dot-FD & Dot & Dot-FD \\ \midrule    

        
        $s$=100 & 0.00 & 0.00 & 52.89 & 53.75 & 0.00 & 0.00 & 0.00 & 0.00 \\ 
        
        $s$=50 & 0.00 & 0.00 & 51.23 & 50.12 & 0.00 & 0.00 & 0.00 & 0.00 \\ 
        

        
        $s$=10 & 0.00 & 0.00 & 43.07 & 47.28 & 0.00 & 0.00 & 0.00 & 0.00 \\ 
        \bottomrule

    
    
        \end{tabular}
        }
\end{table}


\newpage

\begin{table}[h!]
    \centering
    \caption{Grid Search Results for VGG11 on CIFAR-10.}  
    \resizebox{0.65\textwidth}{!}{
        \begin{tabular}{c|cc|cc|cc|cc}
        \toprule
        \multirow{2.5}{*} {\emph{$\eta$=0.01}} & \multicolumn{2}{c|}{$E$=5} & \multicolumn{2}{c|}{$E$=10} & \multicolumn{2}{c|}{$E$=15} & \multicolumn{2}{c}{$E$=20}  \\ \cmidrule{2-9}         
        & Dot & Dot-FD & Dot & Dot-FD & Dot & Dot-FD & Dot & Dot-FD \\ \midrule    

        $s$=10 & 0.00 & 0.00 & 80.18 & 79.85 & 0.00 & 0.00 & 0.00 & 0.00\\ 
        
        $s$=5 & 0.00 & 0.00 & 77.92 & 77.78 & 0.00 & 0.00 & 0.00 & 0.00\\
        
        $s$=2 & 0.00 & 0.00 & 66.65 & 66.06 & 0.00 & 0.00 & 0.00 & 0.00\\ \midrule
        
        \multirow{2.5}{*} {\emph{$\eta$=0.03}} & \multicolumn{2}{c|}{$E$=5} & \multicolumn{2}{c|}{$E$=10} & \multicolumn{2}{c|}{$E$=15} & \multicolumn{2}{c}{$E$=20}  \\ \cmidrule{2-9}         
        & Dot & Dot-FD & Dot & Dot-FD & Dot & Dot-FD & Dot & Dot-FD \\ \midrule    

        $s$=10 & 0.00 & 0.00 & 81.46 & 81.39 & 0.00 & 0.00 & 0.00 & 0.00\\ 
        
        $s$=5 & 0.00 & 0.00 & 80.42 & 79.80 & 0.00 & 0.00 & 0.00 & 0.00\\
        
        $s$=2 & 0.00 & 0.00 & 72.20 & 72.15 & 0.00 & 0.00 & 0.00 & 0.00\\ \midrule


        \multirow{2.5}{*} {\emph{$\eta$=0.05}} & \multicolumn{2}{c|}{$E$=5} & \multicolumn{2}{c|}{$E$=10} & \multicolumn{2}{c|}{$E$=15} & \multicolumn{2}{c}{$E$=20}  \\ \cmidrule{2-9}         
        & Dot & Dot-FD & Dot & Dot-FD & Dot & Dot-FD & Dot & Dot-FD \\ \midrule    

        $s$=10 & 0.00 & 0.00 & 82.31 & 82.03 & 0.00 & 0.00 & 0.00 & 0.00\\ 
        
        $s$=5 & 0.00 & 0.00 & 81.09 & 80.80 & 0.00 & 0.00 & 0.00 & 0.00\\
        
        $s$=2 & 0.00 & 0.00 & 74.03 & 74.27 & 0.00 & 0.00 & 0.00 & 0.00\\ \midrule
        
        
        \multirow{2.5}{*} {\emph{$\eta$=0.1}} & \multicolumn{2}{c|}{$E$=5} & \multicolumn{2}{c|}{$E$=10} & \multicolumn{2}{c|}{$E$=15} & \multicolumn{2}{c}{$E$=20}  \\ \cmidrule{2-9}         
        & Dot & Dot-FD & Dot & Dot-FD & Dot & Dot-FD & Dot & Dot-FD \\ \midrule    

        $s$=10 & 0.00 & 0.00 & 82.78 & 82.57 & 0.00 & 0.00 & 0.00 & 0.00\\ 
        
        $s$=5 & 0.00 & 0.00 & 81.85 & 81.99 & 0.00 & 0.00 & 0.00 & 0.00\\
        
        $s$=2 & 0.00 & 0.00 & 74.94 & 75.61 & 0.00 & 0.00 & 0.00 & 0.00\\ \midrule

        \multirow{2.5}{*} {\emph{$\eta$=0.15}} & \multicolumn{2}{c|}{$E$=5} & \multicolumn{2}{c|}{$E$=10} & \multicolumn{2}{c|}{$E$=15} & \multicolumn{2}{c}{$E$=20}  \\ \cmidrule{2-9}         
        & Dot & Dot-FD & Dot & Dot-FD & Dot & Dot-FD & Dot & Dot-FD \\ \midrule    

        $s$=10 & 0.00 & 0.00 & 83.10 & 83.25 & 0.00 & 0.00 & 0.00 & 0.00\\ 
        
        $s$=5 & 0.00 & 0.00 & 82.37 & 81.94 & 0.00 & 0.00 & 0.00 & 0.00\\
        
        $s$=2 & 0.00 & 0.00 & 75.50 & 76.42 & 0.00 & 0.00 & 0.00 & 0.00\\ \midrule

        \multirow{2.5}{*} {\emph{$\eta$=0.2}} & \multicolumn{2}{c|}{$E$=5} & \multicolumn{2}{c|}{$E$=10} & \multicolumn{2}{c|}{$E$=15} & \multicolumn{2}{c}{$E$=20}  \\ \cmidrule{2-9}         
        & Dot & Dot-FD & Dot & Dot-FD & Dot & Dot-FD & Dot & Dot-FD \\ \midrule    

        $s$=10 & 0.00 & 0.00 & 83.15 & 83.34 & 0.00 & 0.00 & 0.00 & 0.00\\ 
        
        $s$=5 & 0.00 & 0.00 & 82.56 & 82.97 & 0.00 & 0.00 & 0.00 & 0.00\\
        
        $s$=2 & 0.00 & 0.00 & 75.41 & 76.12 & 0.00 & 0.00 & 0.00 & 0.00\\ \midrule


        \multirow{2.5}{*} {\emph{$\eta$=0.25}} & \multicolumn{2}{c|}{$E$=5} & \multicolumn{2}{c|}{$E$=10} & \multicolumn{2}{c|}{$E$=15} & \multicolumn{2}{c}{$E$=20}  \\ \cmidrule{2-9}         
        & Dot & Dot-FD & Dot & Dot-FD & Dot & Dot-FD & Dot & Dot-FD \\ \midrule    

        $s$=10 & 0.00 & 0.00 & \textbf{83.33} & 83.89 & 0.00 & 0.00 & 0.00 & 0.00\\ 
        
        $s$=5 & 0.00 & 0.00 & \textbf{82.32} & 82.71 & 0.00 & 0.00 & 0.00 & 0.00\\
        
        $s$=2 & 0.00 & 0.00 & \textbf{76.48} & 76.87 & 0.00 & 0.00 & 0.00 & 0.00\\ \midrule
        
        \multirow{2.5}{*} {\emph{$\eta$=0.3}} & \multicolumn{2}{c|}{$E$=5} & \multicolumn{2}{c|}{$E$=10} & \multicolumn{2}{c|}{$E$=15} & \multicolumn{2}{c}{$E$=20}  \\ \cmidrule{2-9}         
        & Dot & Dot-FD & Dot & Dot-FD & Dot & Dot-FD & Dot & Dot-FD \\ \midrule    

        $s$=10 & 0.00 & 0.00 & 83.12 & 84.28 & 0.00 & 0.00 & 0.00 & 0.00\\ 
        
        $s$=5 & 0.00 & 0.00 & 82.74 & 82.93 & 0.00 & 0.00 & 0.00 & 0.00\\
        
        $s$=2 & 0.00 & 0.00 & 74.23 & 77.53 & 0.00 & 0.00 & 0.00 & 0.00\\ \midrule
        
        \multirow{2.5}{*} {\emph{$\eta$=0.35}} & \multicolumn{2}{c|}{$E$=5} & \multicolumn{2}{c|}{$E$=10} & \multicolumn{2}{c|}{$E$=15} & \multicolumn{2}{c}{$E$=20}  \\ \cmidrule{2-9}         
        & Dot & Dot-FD & Dot & Dot-FD & Dot & Dot-FD & Dot & Dot-FD \\ \midrule    

        $s$=10 & 0.00 & 0.00 & 0.00 & \textbf{84.19} & 0.00 & 0.00 & 0.00 & 0.00\\ 
        
        $s$=5 & 0.00 & 0.00 & 0.00 & \textbf{83.29} & 0.00 & 0.00 & 0.00 & 0.00\\
        
        $s$=2 & 0.00 & 0.00 & 74.96 & \textbf{77.56} & 0.00 & 0.00 & 0.00 & 0.00\\  \midrule      

        \multirow{2.5}{*} {\emph{$\eta$=0.4}} & \multicolumn{2}{c|}{$E$=5} & \multicolumn{2}{c|}{$E$=10} & \multicolumn{2}{c|}{$E$=15} & \multicolumn{2}{c}{$E$=20}  \\ \cmidrule{2-9}         
        & Dot & Dot-FD & Dot & Dot-FD & Dot & Dot-FD & Dot & Dot-FD \\ \midrule    

        $s$=10 & 0.00 & 0.00 & 0.00 & 84.31 & 0.00 & 0.00 & 0.00 & 0.00\\ 
        
        $s$=5 & 0.00 & 0.00 & 0.00 & 83.24 & 0.00 & 0.00 & 0.00 & 0.00\\
        
        $s$=2 & 0.00 & 0.00 & 73.54 & 77.54 & 0.00 & 0.00 & 0.00 & 0.00\\  \bottomrule    

        % \multirow{2.5}{*} {\emph{$\eta$=0.45}} & \multicolumn{2}{c|}{$E$=5} & \multicolumn{2}{c|}{$E$=10} & \multicolumn{2}{c|}{$E$=15} & \multicolumn{2}{c}{$E$=20}  \\ \cmidrule{2-9}         
        % & Dot & Dot-FD & Dot & Dot-FD & Dot & Dot-FD & Dot & Dot-FD \\ \midrule    

        % $s$=10 & 0.00 & 0.00 & 0.00 & 84.07 & 0.00 & 0.00 & 0.00 & 0.00\\ 
        
        % $s$=5 & 0.00 & 0.00 & 0.00 & 83.74 & 0.00 & 0.00 & 0.00 & 0.00\\
        
        % $s$=2 & 0.00 & 0.00 & 72.87 & 77.35 & 0.00 & 0.00 & 0.00 & 0.00\\  \midrule     


        % \multirow{2.5}{*} {\emph{$\eta$=0.5}} & \multicolumn{2}{c|}{$E$=5} & \multicolumn{2}{c|}{$E$=10} & \multicolumn{2}{c|}{$E$=15} & \multicolumn{2}{c}{$E$=20}  \\ \cmidrule{2-9}         
        % & Dot & Dot-FD & Dot & Dot-FD & Dot & Dot-FD & Dot & Dot-FD \\ \midrule    

        % $s$=10 & 0.00 & 0.00 & 0.00 & 84.32 & 0.00 & 0.00 & 0.00 & 0.00\\ 
        
        % $s$=5 & 0.00 & 0.00 & 0.00 & 83.48 & 0.00 & 0.00 & 0.00 & 0.00\\
        
        % $s$=2 & 0.00 & 0.00 & 68.32 & 77.10 & 0.00 & 0.00 & 0.00 & 0.00\\
        \end{tabular}
        } 
\end{table}



\newpage

\subsection{FedNCP vs. FedNCP-FD}

\begin{table}[htp]
    \centering
    \caption{Grid Search Results for MobileNet on CIFAR-100.}
    \resizebox{0.6\textwidth}{!}{
        \begin{tabular}{c|cc|cc|cc|cc}
        \toprule
        \multirow{2.5}{*} {\emph{$\eta$=1.0}} & \multicolumn{2}{c|}{$E$=1} & \multicolumn{2}{c|}{$E$=3} & \multicolumn{2}{c|}{$E$=5} & \multicolumn{2}{c}{$E$=10} \\ \cmidrule{2-9}         
        & NCP & NCP-FD & NCP & NCP-FD & NCP & NCP-FD & NCP & NCP-FD \\ \midrule    

        
        $s$=100 & 37.05 & 34.62 & 52.08 & 48.32 & 46.00 & 44.97 & 41.66 & 42.01 \\ 
        
        $s$=50 & 33.88 & 34.14 & 48.33 & 49.40 & 43.72 & 44.86 & 39.58 & 39.96 \\ 
        

        % $s$=20 & 0.00 & 0.00 & 45.46 & 47.11 & 0.00 & 0.00 & 0.00 & 0.00 \\  
        
        $s$=10 & 23.84 & 0.00 & 40.94 & 43.81 & 40.54 & 0.00 & 33.76 & 0.00 \\    
        \midrule
        
        \multirow{2.5}{*} {\emph{$\eta$=2.0}} & \multicolumn{2}{c|}{$E$=1} & \multicolumn{2}{c|}{$E$=3} & \multicolumn{2}{c|}{$E$=5} & \multicolumn{2}{c}{$E$=10} \\ \cmidrule{2-9}         
        & NCP & NCP-FD & NCP & NCP-FD & NCP & NCP-FD & NCP & NCP-FD \\ \midrule    

        
        $s$=100 & 42.45 & 41.92 & 51.60 & 49.67 & 45.31 & 45.20 & 43.14 & 43.92 \\ 
        
        $s$=50 & 36.64 & 36.64 & 51.24 & 49.67 & 46.74 & 44.96 & 42.99 & 42.52 \\ 
        

        % $s$=20 & 0.00 & 0.00 & 47.92 & 48.74 & 0.00 & 0.00 & 0.00 & 0.00 \\  
        
        $s$=10 & 26.79 & 0.00 & 38.94 & 47.85 & 41.73 & 0.00 & 34.543 & 0.00 \\    
        \midrule

        \multirow{2.5}{*} {\emph{$\eta$=2.5}} & \multicolumn{2}{c|}{$E$=1} & \multicolumn{2}{c|}{$E$=3} & \multicolumn{2}{c|}{$E$=5} & \multicolumn{2}{c}{$E$=10} \\ \cmidrule{2-9}         
        & NCP & NCP-FD & NCP & NCP-FD & NCP & NCP-FD & NCP & NCP-FD \\ \midrule    

        
        $s$=100 & 45.25 & 42.73 & 49.86 & 50.87 & 46.24 & 47.70 & 43.66 & 42.92 \\ 
        
        $s$=50 & 40.80 & 38.08 & 50.78 & 50.75 & 47.82 & 47.58 & 42.09 & 42.31 \\ 
        

        % $s$=20 & 0.00 & 0.00 & 48.17 & 49.88 & 0.00 & 0.00 & 0.00 & 0.00 \\  
        
        $s$=10 & 30.20 & 0.00 & 44.47 & 48.29 & 40.22 & 0.00 & 33.62 & 0.00 \\    
        \midrule
        

        
        \multirow{2.5}{*} {\emph{$\eta$=3.0}} & \multicolumn{2}{c|}{$E$=1} & \multicolumn{2}{c|}{$E$=3} & \multicolumn{2}{c|}{$E$=5} & \multicolumn{2}{c}{$E$=10} \\ \cmidrule{2-9}         
        & NCP & NCP-FD & NCP & NCP-FD & NCP & NCP-FD & NCP & NCP-FD \\ \midrule    

        
        $s$=100 & 44.67 & 43.89 & \textbf{52.17} & \textbf{52.65} & 48.42 & 48.66 & 43.67 & 44.03 \\ 
        
        $s$=50 & 42.08 & 39.72 & \textbf{49.87} & \textbf{51.24} & 47.47 & 47.27 & 42.27 & 42.12 \\ 
        

        % $s$=20 & 0.00 & 0.00 & \textbf{48.28} & \textbf{51.03} & 0.00 & 0.00 & 0.00 & 0.00 \\  
        
        $s$=10 & 28.60 & 0.00 & \textbf{44.81} & \textbf{49.27} & 43.58 & 0.00 & 29.56 & 0.00 \\    
        \midrule

        \multirow{2.5}{*} {\emph{$\eta$=3.5}} & \multicolumn{2}{c|}{$E$=1} & \multicolumn{2}{c|}{$E$=3} & \multicolumn{2}{c|}{$E$=5} & \multicolumn{2}{c}{$E$=10} \\ \cmidrule{2-9}         
        & NCP & NCP-FD & NCP & NCP-FD & NCP & NCP-FD & NCP & NCP-FD \\ \midrule    

        
        $s$=100 & 45.86 & 43.89 & 52.77 & 49.76 & 48.50 & 48.66 & 43.81 & 44.03 \\ 
        
        $s$=50 & 40.84 & 40.38 & 51.48 & 51.92 & 46.84 & 48.98 & 43.24 & 43.75 \\ 
        

        % $s$=20 & 0.00 & 0.00 & 47.20 & 50.05 & 0.00 & 0.00 & 0.00 & 0.00 \\  
        
        $s$=10 & 29.23 & 0.00 & 35.97 & 48.73 & 40.55 & 0.00 & 31.21 & 0.00 \\    
        \midrule

        \multirow{2.5}{*} {\emph{$\eta$=4.0}} & \multicolumn{2}{c|}{$E$=1} & \multicolumn{2}{c|}{$E$=3} & \multicolumn{2}{c|}{$E$=5} & \multicolumn{2}{c}{$E$=10} \\ \cmidrule{2-9}         
        & NCP & NCP-FD & NCP & NCP-FD & NCP & NCP-FD & NCP & NCP-FD \\ \midrule    

        
        $s$=100 & 45.73 & 43.64 & 52.49 & 52.65 & 49.08 & 48.97 & 43.78 & 43.68 \\ 
        
        $s$=50 & 41.85 & 41.06 & 52.77 & 51.67 & 48.50 & 50.63 & 44.04 & 42.79 \\ 
        

        % $s$=20 & 0.00 & 0.00 & 48.17 & 50.89 & 0.00 & 0.00 & 0.00 & 0.00 \\  
        
        $s$=10 & 30.98 & 0.00 & 41.45 & 48.76 & 38.14 & 0.00 & 28.27 & 0.00 \\    
        \bottomrule

    
    
        \end{tabular}
        }
\end{table}

\newpage

\begin{table}[h!]
    \centering
    \caption{Grid Search Results for VGG11 on CIFAR-10.}  
    \resizebox{0.65\textwidth}{!}{
        \begin{tabular}{c|cc|cc|cc|cc}
        \toprule
        \multirow{2.5}{*} {\emph{$\eta$=0.01}} & \multicolumn{2}{c|}{$E$=5} & \multicolumn{2}{c|}{$E$=10} & \multicolumn{2}{c|}{$E$=15} & \multicolumn{2}{c}{$E$=20}  \\ \cmidrule{2-9}         
        & NCP & NCP-FD & NCP & NCP-FD & NCP & NCP-FD & NCP & NCP-FD \\ \midrule 

        $s$=10 & 77.87 & 0.00 & 80.77 & 80.65 & 80.77 & 0.00 & 80.42 & 0.00\\ 
        
        $s$=5 & 72.53 & 0.00 & 78.94 & 78.61 & 79.80 & 0.00 & 79.09 & 0.00\\
        
        $s$=2 & 58.06 & 0.00 & 68.68 & 68.65 & 71.51 & 0.00 & 72.17 & 0.00\\ \midrule
        
        \multirow{2.5}{*} {\emph{$\eta$=0.03}} & \multicolumn{2}{c|}{$E$=5} & \multicolumn{2}{c|}{$E$=10} & \multicolumn{2}{c|}{$E$=15} & \multicolumn{2}{c}{$E$=20}  \\ \cmidrule{2-9}         
        & NCP & NCP-FD & NCP & NCP-FD & NCP & NCP-FD & NCP & NCP-FD \\ \midrule     

        $s$=10 & 81.67 & 0.00 & 81.85 & 82.01 & 81.54 & 0.00 & 80.80 & 0.00\\ 
        
        $s$=5 & 78.15 & 0.00 & 81.07 & 80.74 & 81.36 & 0.00 & 80.83 & 0.00\\
        
        $s$=2 & 63.55 & 0.00 & 73.98 & 74.10 & 75.35 & 0.00 & 75.68 & 0.00\\ \midrule


        \multirow{2.5}{*} {\emph{$\eta$=0.05}} & \multicolumn{2}{c|}{$E$=5} & \multicolumn{2}{c|}{$E$=10} & \multicolumn{2}{c|}{$E$=15} & \multicolumn{2}{c}{$E$=20}  \\ \cmidrule{2-9}         
        & NCP & NCP-FD & NCP & NCP-FD & NCP & NCP-FD & NCP & NCP-FD \\ \midrule 
        $s$=10 & 82.72 & 0.00 & 82.55 & 82.86 & 82.40 & 0.00 & 81.94 & 0.00\\ 
        
        $s$=5 & 79.81 & 0.00 & 81.22 & 81.89 & 82.12 & 0.00 & 81.45 & 0.00\\
        
        $s$=2 & 65.28 & 0.00 & 75.05 & 75.49 & 76.39 & 0.00 & 77.03 & 0.00\\ \midrule
        
        
        \multirow{2.5}{*} {\emph{$\eta$=0.1}} & \multicolumn{2}{c|}{$E$=5} & \multicolumn{2}{c|}{$E$=10} & \multicolumn{2}{c|}{$E$=15} & \multicolumn{2}{c}{$E$=20}  \\ \cmidrule{2-9}         
        & NCP & NCP-FD & NCP & NCP-FD & NCP & NCP-FD & NCP & NCP-FD \\ \midrule     

        $s$=10 & 83.32 & 0.00 & 83.24 & 82.90 & 83.59 & 0.00 & 83.23 & 0.00\\ 
        
        $s$=5 & 80.68 & 0.00 & 82.46 & 82.38 & 83.08 & 0.00 & 82.57 & 0.00\\
        
        $s$=2 & 67.37 & 0.00 & 76.55 & 76.83 & 77.70 & 0.00 & 78.27 & 0.00\\ \midrule

        \multirow{2.5}{*} {\emph{$\eta$=0.15}} & \multicolumn{2}{c|}{$E$=5} & \multicolumn{2}{c|}{$E$=10} & \multicolumn{2}{c|}{$E$=15} & \multicolumn{2}{c}{$E$=20}  \\ \cmidrule{2-9}         
        & NCP & NCP-FD & NCP & NCP-FD & NCP & NCP-FD & NCP & NCP-FD \\ \midrule     

        $s$=10 & 83.35 & 0.00 & \textbf{83.90} & 84.29 & 83.43 & 0.00 & 83.46 & 0.00\\ 
        
        $s$=5 & 81.24 & 0.00 & \textbf{82.34} & 82.98 & 82.84 & 0.00 & 82.79 & 0.00\\
        
        $s$=2 & 66.38 & 0.00 & \textbf{76.93} & 77.92 & 78.62 & 0.00 & 78.16 & 0.00\\ \midrule

        \multirow{2.5}{*} {\emph{$\eta$=0.2}} & \multicolumn{2}{c|}{$E$=5} & \multicolumn{2}{c|}{$E$=10} & \multicolumn{2}{c|}{$E$=15} & \multicolumn{2}{c}{$E$=20}  \\ \cmidrule{2-9}         
        & NCP & NCP-FD & NCP & NCP-FD & NCP & NCP-FD & NCP & NCP-FD \\ \midrule 

        $s$=10 & 83.45 & 0.00 & 83.63 & 83.53 & 83.65 & 0.00 & 83.70 & 0.00\\ 
        
        $s$=5 & 80.99 & 0.00 & 82.95 & 83.63 & 83.25 & 0.00 & 83.31 & 0.00\\
        
        $s$=2 & 64.70 & 0.00 & 76.36 & 77.30 & 78.07 & 0.00 & 78.40 & 0.00\\ \midrule


        \multirow{2.5}{*} {\emph{$\eta$=0.25}} & \multicolumn{2}{c|}{$E$=5} & \multicolumn{2}{c|}{$E$=10} & \multicolumn{2}{c|}{$E$=15} & \multicolumn{2}{c}{$E$=20}  \\ \cmidrule{2-9}         
        & NCP & NCP-FD & NCP & NCP-FD & NCP & NCP-FD & NCP & NCP-FD \\ \midrule    

        $s$=10 & 83.56 & 0.00 & 82.98 & \textbf{84.30} & 83.87 & 0.00 & 83.94 & 0.00\\ 
        
        $s$=5 & 81.06 & 0.00 & 82.53 & \textbf{83.20} & 83.10 & 0.00 & 83.49 & 0.00\\
        
        $s$=2 & 61.70 & 0.00 & 76.06 & \textbf{77.96} & 77.55 & 0.00 & 78.57 & 0.00\\ \midrule
        
        \multirow{2.5}{*} {\emph{$\eta$=0.3}} & \multicolumn{2}{c|}{$E$=5} & \multicolumn{2}{c|}{$E$=10} & \multicolumn{2}{c|}{$E$=15} & \multicolumn{2}{c}{$E$=20}  \\ \cmidrule{2-9}         
        & NCP & NCP-FD & NCP & NCP-FD & NCP & NCP-FD & NCP & NCP-FD \\ \midrule    

        $s$=10 & 83.80 & 0.00 & 83.10 & 83.93 & 83.40 & 0.00 & 84.24 & 0.00\\ 
        
        $s$=5 & 81.25 & 0.00 & 82.77 & 82.60 & 83.28 & 0.00 & 83.44 & 0.00\\
        
        $s$=2 & 61.35 & 0.00 & 75.16 & 77.45 & 77.66 & 0.00 & 78.43 & 0.00\\ \bottomrule
        
        \end{tabular}
        } 
\end{table}



% \begin{table}[h!]
%     \centering
%     \caption{Grid Search Results for Simple CNN on CIFAR-10.}    
%     \resizebox{0.25\textwidth}{!}{
%         \begin{tabular}{c|cccc}
%         \toprule        
%         {\emph{$\eta$=0.01}} & {$E$=5} & {$E$=10}  & {$E$=15} & {$E$=20}\\ \midrule  
%         Shard 10 & 62.35 & 67.40 & 68.55 & 0.00 \\ 
%         Shard 5 & 57.73 & 61.51 & 64.45 & 0.00 \\ 
%         Shard 3 & 53.10 & 55.19 & 56.84 & 0.00 \\  \midrule

%         {\emph{$\eta$=0.05}} & {$E$=5} & {$E$=10}  & {$E$=15} & {$E$=20}\\ \midrule  
%         Shard 10 & 63.31 & 66.01 & 67.94 & 0.00 \\ 
%         Shard 5 & 61.64 & 62.39 & 65.55 & 0.00 \\ 
%         Shard 3 & 55.45 & 57.75 & 57.75 & 0.00 \\  \midrule


%         {\emph{$\eta$=0.1}} & {$E$=5} & {$E$=10}  & {$E$=15} & {$E$=20}\\ \midrule  
%         Shard 10 & 63.56 & 66.40 & \textbf{67.39} & 0.00 \\ 
%         Shard 5 & 60.62 & 63.26 & \textbf{63.46} & 0.00 \\ 
%         Shard 3 & 54.01 & 57.75 & \textbf{59.03} & 0.00 \\   \midrule

%         {\emph{$\eta$=0.2}} & $E$=5  & {$E$=10}  & {$E$=15} & {$E$=20}\\ \midrule     
%         Shard 10 & 64.14 & 66.34 & 65.58 & 0.00 \\ 
%         Shard 5 & 60.51 & 63.12 & 63.78 & 0.00 \\ 
%         Shard 3 & 52.91 & 54.16 & 54.24 & 0.00 \\  \bottomrule        
%         \end{tabular}
%         }
% \end{table}


% \begin{table}[h!]
%     \centering
%     \caption{Grid Search Results for ResNet18 on CIFAR-10.}    
%     \resizebox{0.25\textwidth}{!}{
%         \begin{tabular}{c|cccc}
%         \toprule        
%         {\emph{$\eta$=0.01}} & {$E$=5} & {$E$=10} & {$E$=15} & {$E$=20}\\ \midrule   
%         Shard 10 & 72.82 & 74.14 & 73.74 & 0.00 \\
%         Shard 5 & 66.43 & 70.71 & 69.84 & 0.00 \\
%         Shard 3 & 60.68 & 64.70 & 65.25 & 0.00 \\ \midrule

%         {\emph{$\eta$=0.05}} & {$E$=5} & {$E$=10} & {$E$=15} & {$E$=20}\\ \midrule   
%         Shard 10 & 78.58 & 78.32 & 77.51 & 0.00 \\
%         Shard 5 & 76.56 & 72.52 & 71.58 & 0.00 \\
%         Shard 3 & 61.98 & 56.16 & 61.33 & 0.00 \\ \midrule


%         {\emph{$\eta$=0.1}} & {$E$=5} & {$E$=10} & {$E$=15} & {$E$=20}\\ \midrule   
%         Shard 10 & \textbf{79.12} & 80.34 & 79.58 & 0.00 \\
%         Shard 5 & \textbf{72.78} & 71.41 & 72.12 & 0.00 \\
%         Shard 3 & \textbf{64.76} & 64.32 & 62.75 & 0.00 \\    \midrule

%         {\emph{$\eta$=0.2}} & {$E$=5} & {$E$=10} & {$E$=15} & {$E$=20}\\ \midrule    
%         Shard 10 & 80.99 & 81.28 & 81.00 & 0.00 \\
%         Shard 5 & 72.60 & 69.13 & 68.94 & 0.00 \\
%         Shard 3 & 61.76 & 62.80 & 57.62 & 0.00 \\   \midrule

%         \end{tabular}
%         }
% \end{table}


\clearpage
\subsection{SphereFed}
We conduct grid searches for SphereFed~\cite{dong2022spherefed} for MobileNet on CIFAR-100. Consequently, in Table ~\ref{apptab:grid_sphere_additional}, we extend the $\eta$ search exclusively for SphereFed to include values $\{0.1, 1.0, 1.5, 3.0, 4.5, 5.0\}$. In summary, the determined optimal hyperparameter $\eta$ values is 4.5.


\begin{table}[htp]
    \centering
    \caption{Grid Search Results for SphereFed with MobileNet on CIFAR-100.}
    \resizebox{0.35\textwidth}{!}{
        \begin{tabular}{c|cccc}
        \toprule

        {\emph{$\eta$=0.1}} & {$E$=1} & {$E$=3} & {$E$=5} & {$E$=10} \\ \midrule         
        $s$=100 & 1.37 & 1.58  & 2.16 & 4.25     \\ 
        
        $s$=50 & 1.30 & 2.10  & 1.73 & 3.84     \\  
        

        % $s$=20 & 0.00 & 2.03  & 0.00 & 0.00 \\ 
        
        $s$=10 & 1.46 & 1.60  & 2.34 & 3.81 \\ 

        
        \midrule

        {\emph{$\eta$=1.0}} & {$E$=1} & {$E$=3} & {$E$=5} & {$E$=10} \\ \midrule         
        $s$=100 & 2.33 & 10.89  & 29.94 & 40.02     \\ 
        
        $s$=50 & 2.27 & 12.08  & 29.39 & 40.87     \\  
        
        % $s$=20 & 0.00 & 10.86  & 0.00 & 0.00 \\ 
        
        $s$=10 & 1.70 & 8.62  & 23.38 & 32.64 \\ 

        
        \midrule
        
        % {\emph{$\eta$=1.5}} & {$E$=1} & {$E$=3} & {$E$=5} & {$E$=10} \\ \midrule         
        % $s$=100 & 2.84 & 18.86  & 44.40 & 40.32     \\ 
        
        % $s$=50 & 2.81 & 21.88  & 41.91 & 42.18     \\  
        
        % $s$=30 & 3.23 & 17.91  & 36.82 & 39.51     \\ \midrule
        
        {\emph{$\eta$=3.0}} & {$E$=1} & {$E$=3} & {$E$=5} & {$E$=10} \\ \midrule

        
        $s$=100 & 6.37 & 40.72  & 47.44 & 42.15     \\ 
        
        $s$=50 & 5.05 & 39.75  & 45.56 & 42.61     \\  
        
        
        % $s$=20 & 0.00 & 39.47  & 0.00 & 0.00 \\ 

        $s$=10 & 4.87 & 32.97  & 40.84 & 41.12     \\
  
        \midrule

        % {\emph{$\eta$=4.0}} & {$E$=1} & {$E$=3} & {$E$=5} & {$E$=10} \\ \midrule     
         
        % $s$=100 & 7.67 & 48.06  & 49.03 & 41.71     \\ 
        
        % $s$=50 & 8.42 & 49.41  & 48.42 & 42.54     \\  
        
        % $s$=30 & 8.97 & 42.12  & 46.25 & 41.72     \\  \midrule
        
        
        % {\emph{$\eta$=4.5}} & {$E$=1} & {$E$=3} & {$E$=5} & {$E$=10} \\ \midrule     
         
        % $s$=100 & 9.43 & 49.14  & \textbf{49.51} & 43.19     \\ 
        
        % $s$=50 & 8.19 & 47.55  & \textbf{48.05} & 42.42     \\ 
        
        % $s$=30 & 9.08 & 44.41  & 48.99 & 43.49     \\
        % $s$=10 & 0.00 & 0.00  & 0.00 & 0.00     \\
        
        % \midrule


        {\emph{$\eta$=5.0}} & {$E$=1} & {$E$=3} & {$E$=5} & {$E$=10} \\ \midrule              
        $s$=100 & 10.58 & 49.89  & 49.29 & 36.07     \\ 
        
        $s$=50 & 10.95 & 49.88  & 48.08 & 38.49     \\  
        
        % $s$=20 & 0.00 & 46.50  & 0.00 & 0.00 \\ 

        $s$=10 & 8.26 & 42.25  & 43.26 & 38.76 \\        
        
        \midrule


        {\emph{$\eta$=5.5}} & {$E$=1} & {$E$=3} & {$E$=5} & {$E$=10} \\ \midrule     
         
        $s$=100 & 11.41 & 50.33  & 48.93 & 42.72     \\ 
        
        $s$=50 & 11.38 & 50.66  & 49.64 & 43.81     \\  
        
        % $s$=20 & 0.00 & 46.19  & 0.00 & 0.00 \\ 
        
        $s$=10 & 8.84 & 41.93  & 43.52 & 36.83     \\
        
        \midrule

        {\emph{$\eta$=6.0}} & {$E$=1} & {$E$=3} & {$E$=5} & {$E$=10} \\ \midrule     
         
        $s$=100 & 12.15 & 51.31  & 49.73 & 40.59     \\ 
        
        $s$=50 & 12.36 & 50.99  & 49.49 & 42.07     \\  
        
        % $s$=20 & 0.00 & 47.59  & 0.00 & 0.00 \\ 
        
        $s$=10 & 10.00 & 42.06  & 41.93 & 38.59     \\
        
        \midrule

        {\emph{$\eta$=6.5}} & {$E$=1} & {$E$=3} & {$E$=5} & {$E$=10} \\ \midrule     
         
        $s$=100 & 14.01 & \textbf{52.07}  & 49.67 & 43.96     \\ 
        
        $s$=50 & 14.23 & \textbf{50.86}  & 49.66 & 41.75     \\  
        

        % $s$=20 & 0.00 & 47.73  & 0.00 & 0.00 \\ 

        $s$=10 & 11.06 & \textbf{43.90}  & 42.60 & 36.22     \\
        
        \midrule

        {\emph{$\eta$=7.0}} & {$E$=1} & {$E$=3} & {$E$=5} & {$E$=10} \\ \midrule     
         
        $s$=100 & 15.41 & 51.45  & 49.90 & 43.50     \\ 
        
        $s$=50 & 15.37 & 51.55  & 50.50 & 43.53     \\  
        
        % $s$=20 & 0.00 & 49.14  & 0.00 & 0.00 \\ 
        
        $s$=10 & 13.10 & 43.88  & 42.10 & 33.56     \\
        
        \bottomrule
        
        
        \end{tabular}
        }
        \label{apptab:grid_sphere_additional}

\end{table}



\newpage

\begin{table}[h!]
    \centering
    \caption{Grid Search Results for VGG on CIFAR-10.}    
    \resizebox{0.4\textwidth}{!}{
        \begin{tabular}{c|cccc}
        \toprule        
        {\emph{$\eta$=0.01}} & {$E$=5} & {$E$=10}  & {$E$=15} & {$E$=20}\\ \midrule  
        $s$=10 & 66.01 & 75.58 & 77.94 & 77.96 \\ 
        $s$=5 & 60.51 & 71.78 & 75.19 & 76.47 \\ 
        % $s$=3 & 56.35 & 67.02 & 71.66 & 73.19 \\ 
        $s$=2 & 52.28 & 60.53 & 65.77 & 68.48 \\ \midrule

        {\emph{$\eta$=0.1}} & {$E$=5} & {$E$=10}  & {$E$=15} & {$E$=20}\\ \midrule    
        $s$=10 & 81.07 & 81.15 & 80.97 & 80.19 \\ 
        $s$=5 & 77.92 & 80.35 & 80.58 & 80.56 \\  
        % $s$=3 & 70.43 & 76.95 & 77.24 & 77.07 \\         
        $s$=2 & 63.90 & 73.30 & 74.62 & 74.46 \\ \midrule

        {\emph{$\eta$=0.2}} & {$E$=5} & {$E$=10}  & {$E$=15} & {$E$=20}\\ \midrule   
        $s$=10 & 82.67 & 82.97 & 82.02 & 82.23 \\ 
        $s$=5 & 80.00 & 81.62 & 82.68 & 82.25 \\ 
        % $s$=3 & 72.64 & 77.90 & 79.19 & 78.98 \\        
        $s$=2 & 67.32 & 75.93 & 75.94 & 75.92 \\ \midrule
        {\emph{$\eta$=0.3}} & {$E$=5} & {$E$=10}  & {$E$=15} & {$E$=20}\\ \midrule   
        $s$=10 & 83.56 & 83.33 & 83.36 & 83.17 \\ 
        $s$=5 & 80.99 & 82.69 & 82.69 & 83.11 \\ 
        % $s$=3 & 74.47 & 78.75 & 79.39 & 80.04 \\        
        $s$=2 & 69.25 & 76.22 & 77.09 & 76.83 \\ \midrule
        {\emph{$\eta$=0.4}} & {$E$=5} & {$E$=10}  & {$E$=15} & {$E$=20}\\ \midrule    
        $s$=10 & 83.92 & 84.03 & 83.91 & 83.78 \\ 
        $s$=5 & 81.18 & 82.98 & 83.05 & 83.45 \\ 
        % $s$=3 & 75.17 & 79.38 & 79.85 & 80.10 \\        
        $s$=2 & 69.06 & 77.35 & 77.79 & 77.72 \\ \midrule
        {\emph{$\eta$=0.45}} & {$E$=5} & {$E$=10}  & {$E$=15} & {$E$=20}\\ \midrule    
        $s$=10 & 83.83 & 83.98 & 84.46 & 84.64 \\ 
        $s$=5 & 81.53 & 83.13 & 83.90 & 83.50 \\ 
        % $s$=3 & 75.56 & 79.26 & 80.44 & 80.42 \\         
        $s$=2 & 70.50 & 77.26 & 77.86 & 78.01 \\ \midrule      
        {\emph{$\eta$=0.5}} & {$E$=5} & {$E$=10}  & {$E$=15} & {$E$=20}\\ \midrule    
        $s$=10 & 83.91 & 84.43 & 84.39 & 84.71 \\ 
        $s$=5 & 81.86 & 83.26 & 83.68 & 84.09 \\ 
        % $s$=3 & 75.92 & \textbf{79.94} & 80.06 & 80.90 \\         
        $s$=2 & 70.30 & 77.37 & 78.45 & 77.87 \\ \midrule
        {\emph{$\eta$=0.55}} & {$E$=5} & {$E$=10}  & {$E$=15} & {$E$=20}\\ \midrule    
        $s$=10 & 83.87 & \textbf{84.40} & 84.96 & 84.82 \\ 
        $s$=5 & 81.76 & \textbf{83.51} & 83.79 & 83.90 \\ 
        % $s$=3 & 75.42 & 79.65 & 80.28 & 80.41 \\         
        $s$=2 & 70.34 & \textbf{77.70} & 78.24 & 77.78 \\ \midrule              
        {\emph{$\eta$=0.6}} & {$E$=5} & {$E$=10}  & {$E$=15} & {$E$=20}\\ \midrule    
        $s$=10 & 84.35 & 84.35 & 85.07 & 85.02 \\ 
        $s$=5 & 81.93 & 83.36 & 84.41 & 84.28 \\ 
        % $s$=3 & 74.63 & 79.56 & 80.77 & 80.50 \\         
        $s$=2 & 70.20 & 77.60 & 78.89 & 78.00 \\ \midrule      
        {\emph{$\eta$=0.7}} & {$E$=5} & {$E$=10}  & {$E$=15} & {$E$=20}\\ \midrule    
        $s$=10 & 84.57 & 85.22 & 85.17 & 85.24 \\ 
        $s$=5 & 82.35 & 83.62 & 84.34 & 84.05 \\ 
        % $s$=3 & 74.29 & 79.08 & 80.14 & 81.05 \\         
        $s$=2 & 70.09 & 77.16 & 78.81 & 78.10 \\ \bottomrule

        
        % {\emph{$\eta$=0.75}} & {$E$=5} & {$E$=10}  & {$E$=15} & {$E$=20}\\ \midrule    
        % $s$=10 & 84.17 & 84.88 & 85.31 & 85.57 \\ 
        % $s$=5 & 82.37 & 83.44 & 84.00 & 84.34 \\ 
        % % $s$=3 & 75.00 & 78.86 & 80.23 & 80.69 \\          
        % $s$=2 & 68.40 & 77.58 & 78.12 & 77.71 \\ \midrule

        % {\emph{$\eta$=0.8}} & {$E$=5} & {$E$=10}  & {$E$=15} & {$E$=20}\\ \midrule    
        % $s$=10 & 84.70 & 85.14 & 85.14 & 85.25 \\ 
        % $s$=5 & 82.57 & 83.76 & 84.49 & 84.38 \\ 
        % % $s$=3 & 74.08 & 78.25 & 79.60 & 80.31 \\          
        % $s$=2 & 68.67 & 77.38 & 78.53 & 77.61 \\ \midrule 

        % {\emph{$\eta$=0.85}} & {$E$=5} & {$E$=10}  & {$E$=15} & {$E$=20}\\ \midrule    
        % $s$=10 & 84.10 & 85.02 & 85.33 & 86.12 \\ 
        % $s$=5 & 82.43 & 83.81 & 83.94 & 84.43 \\ 
        % % $s$=3 & 74.66 & 78.62 & 80.05 & 79.45 \\          
        % $s$=2 & 68.47 & 76.47 & 78.37 & 77.96 \\ \midrule

        % {\emph{$\eta$=0.9}} & {$E$=5} & {$E$=10}  & {$E$=15} & {$E$=20}\\ \midrule    
        % $s$=10 & 84.64 & 85.04 & 85.64 & 85.35 \\ 
        % $s$=5 & 82.47 & 84.00 & 83.94 & 84.35 \\ 
        % % $s$=3 & 73.64 & 79.77 & 79.51 & 80.19 \\          
        % $s$=2 & 66.56 & 76.70 & 77.79 & 77.39 \\         \bottomrule
        \end{tabular}
        }
\end{table}
\fi
