# Supplementary material for: FedDr+: Stabilizing Dot-regression with Global Feature Distillation for Federated Learning
Source: arXiv:2406.02355 source file (2024-06-04)
Supplement: Supplementary file 3 [file related.tex]

% \section{Additional Related Work}
% \label{sec:appx_related}

% \subsection{Federated Learing}
% \paragraph{Global federated learning.}
% Global Federated Learning (GFL) aims to enhance the performance of a single global model across decentralized clients by addressing data heterogeneity arising from diverse user behaviors. Researchers have explored various methodologies within GFL to create robust models for diverse devices and data sources. These approaches include client drift mitigation~\cite{li2020federated,karimireddy2020scaffold,10077950,NEURIPS2020_564127c0,jhunjhunwala2023fedexp,lee2024fedsol}, aggregation schemes to improve model fusion mechanisms at the server~\cite{wang2020federated, wang2020tackling}, and data sharing techniques introducing public datasets or synthesized data to achieve a more balanced data distribution~\cite{zhao2018federated, lin2020ensemble, luo2021no}.

% \paragraph{Personalized federated learning.}
% Personalized Federated Learning (PFL) focuses on training personalized models for individual clients, adapting to their specific data distributions and tasks. PFL methodologies include decoupling methods that separate the feature extractor and classifier during communication, enabling unique updates for the data distribution of each client~\cite{arivazhagan2019federated, collins2021exploiting, oh2021fedbabu}, modifying local loss functions to improve task performance~\cite{fallah2020personalized, li2021ditto}, and utilizing prototype communication techniques~\cite{tan2022fedproto, xu2023personalized}.

% \subsection{Partial Model Updates in FL}
% \paragraph{Debiasing classifier in FL.}
% Efforts to address data heterogeneity in both GFL and PFL domains have explored differential updates within the model parameters, with a particular focus on the classifier part. For instance, \cite{luo2021no} propose classifier post-calibration with virtual features to tackle a notable bias among classifiers of different local models. \cite{li2021fedrs} introduce the restricted softmax loss for local updates to prevent classifiers from becoming inaccurate when updating for missing classes. Additionally, certain studies~\cite{oh2021fedbabu, dong2022spherefed, li2023no, huang2023neural} suggest the use of fixed classifiers constructed from orthogonal basis vectors during training.

% \paragraph{Feature enhancement in FL.} Recent research~\cite{yu2021fed2, li2021model, li2022federated, shi2022towards} in the context of GFL has focused on aligning feature representations among local models. For instance, \cite{li2021model} introduce the contrastive loss during local iteration to improve feature alignment. Additionally, \cite{shi2022towards} highlights the issue of data heterogeneity leading to severe dimensional collapse in the global model, resulting in representations tending towards lower dimensions. To address this, they propose using a regularization term during local training to mitigate the issue and improve feature alignment. Moreover, some studies ~\cite{tan2022fedproto, xu2023personalized} have explored communication strategies involving feature prototypes to further enhance feature alignment in the context of PFL.


% \subsection{Feature Normalized Model in DL}
% Feature normalized model has been widely adapted in various fields of deep learning (DL), including face recognition~\cite{wang2018additive, savvides2021convex}, regression~\cite{mettes2019hyperspherical}, and federated learning~\cite{dong2022spherefed}, with the aim of enhancing the discriminative power of features. In the several studies~\cite{wang2018additive, dong2022spherefed}, both the feature vectors and classifier weights are normalized to enforce cosine-similarity element logits, restricting the values of each element in the logit vector.
